# Supplementary material for: CoCo-Bench: A Comprehensive Code Benchmark For Multi-task Large Language Model Evaluation
Source: arXiv:2504.20673 source file (2025-04-29)
Supplement: Supplementary file 1 [file 7_correlation_analysis.tex]

\section{Correlation Analysis}
From Figure~\ref{fig:cor1}, we can observe that the CoCo-Score is generally proportional to Human Eval Pass @1, indicating the validity of the CoCo-bench. However, it is evident that some of the high-performing large code models have nearly saturated performance on Human Eval, resulting in a loss of distinction. This suggests that while HumanEval is capable of assessing the basic capabilities of models, it may be insufficient for distinguishing the subtle performance differences among top-tier models.

\begin{figure}[H]
    \centering
    \includegraphics[width=0.8\linewidth]{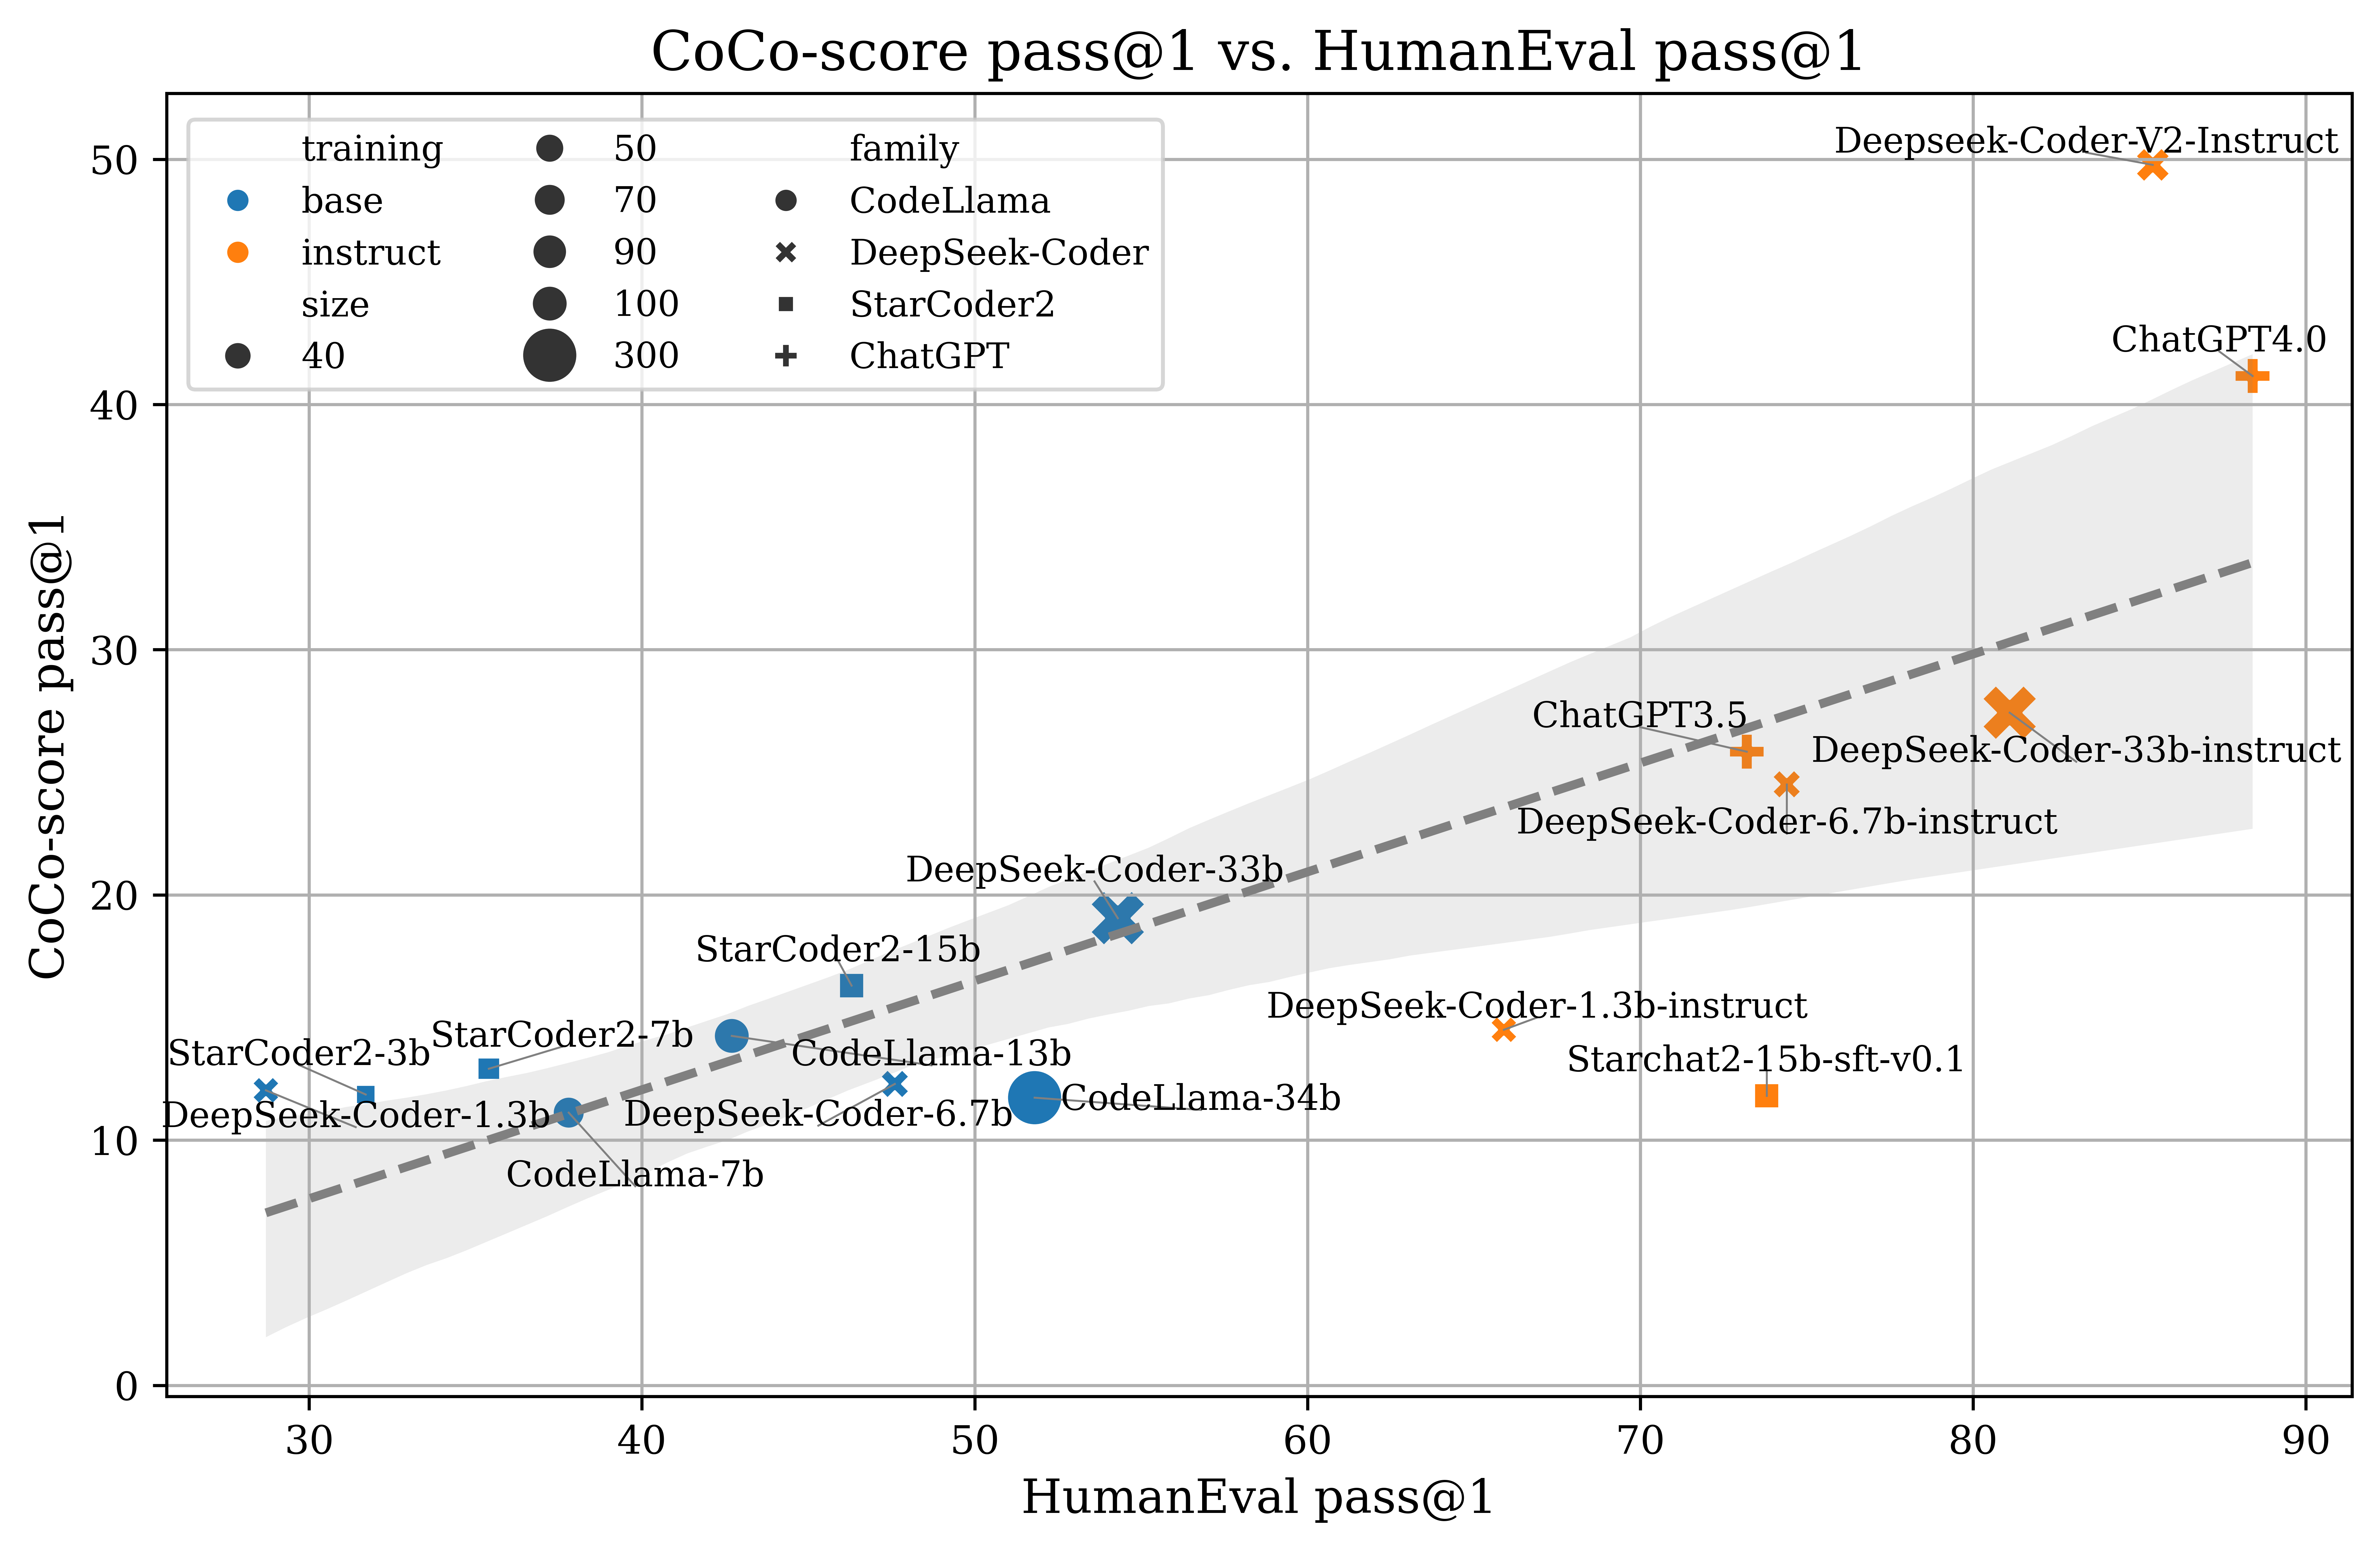}
    \caption{Comparison of CoCo-score pass@1 and HumanEval pass@1 across various models.}
    \label{fig:cor1}
\end{figure}
Similarly, as shown in Figure~\ref{fig:cor2},we selected the CURXEval dataset, which focuses on CU tasks, to demonstrate the validity of our specific task sample design, and it also shows a general proportionality. CU is a relatively challenging task for large code models, which results in most models having lower pass@1 rates on both CoCo-Bench and CURXEval.

\begin{figure}[H]
    \centering
    \includegraphics[width=0.8\linewidth]{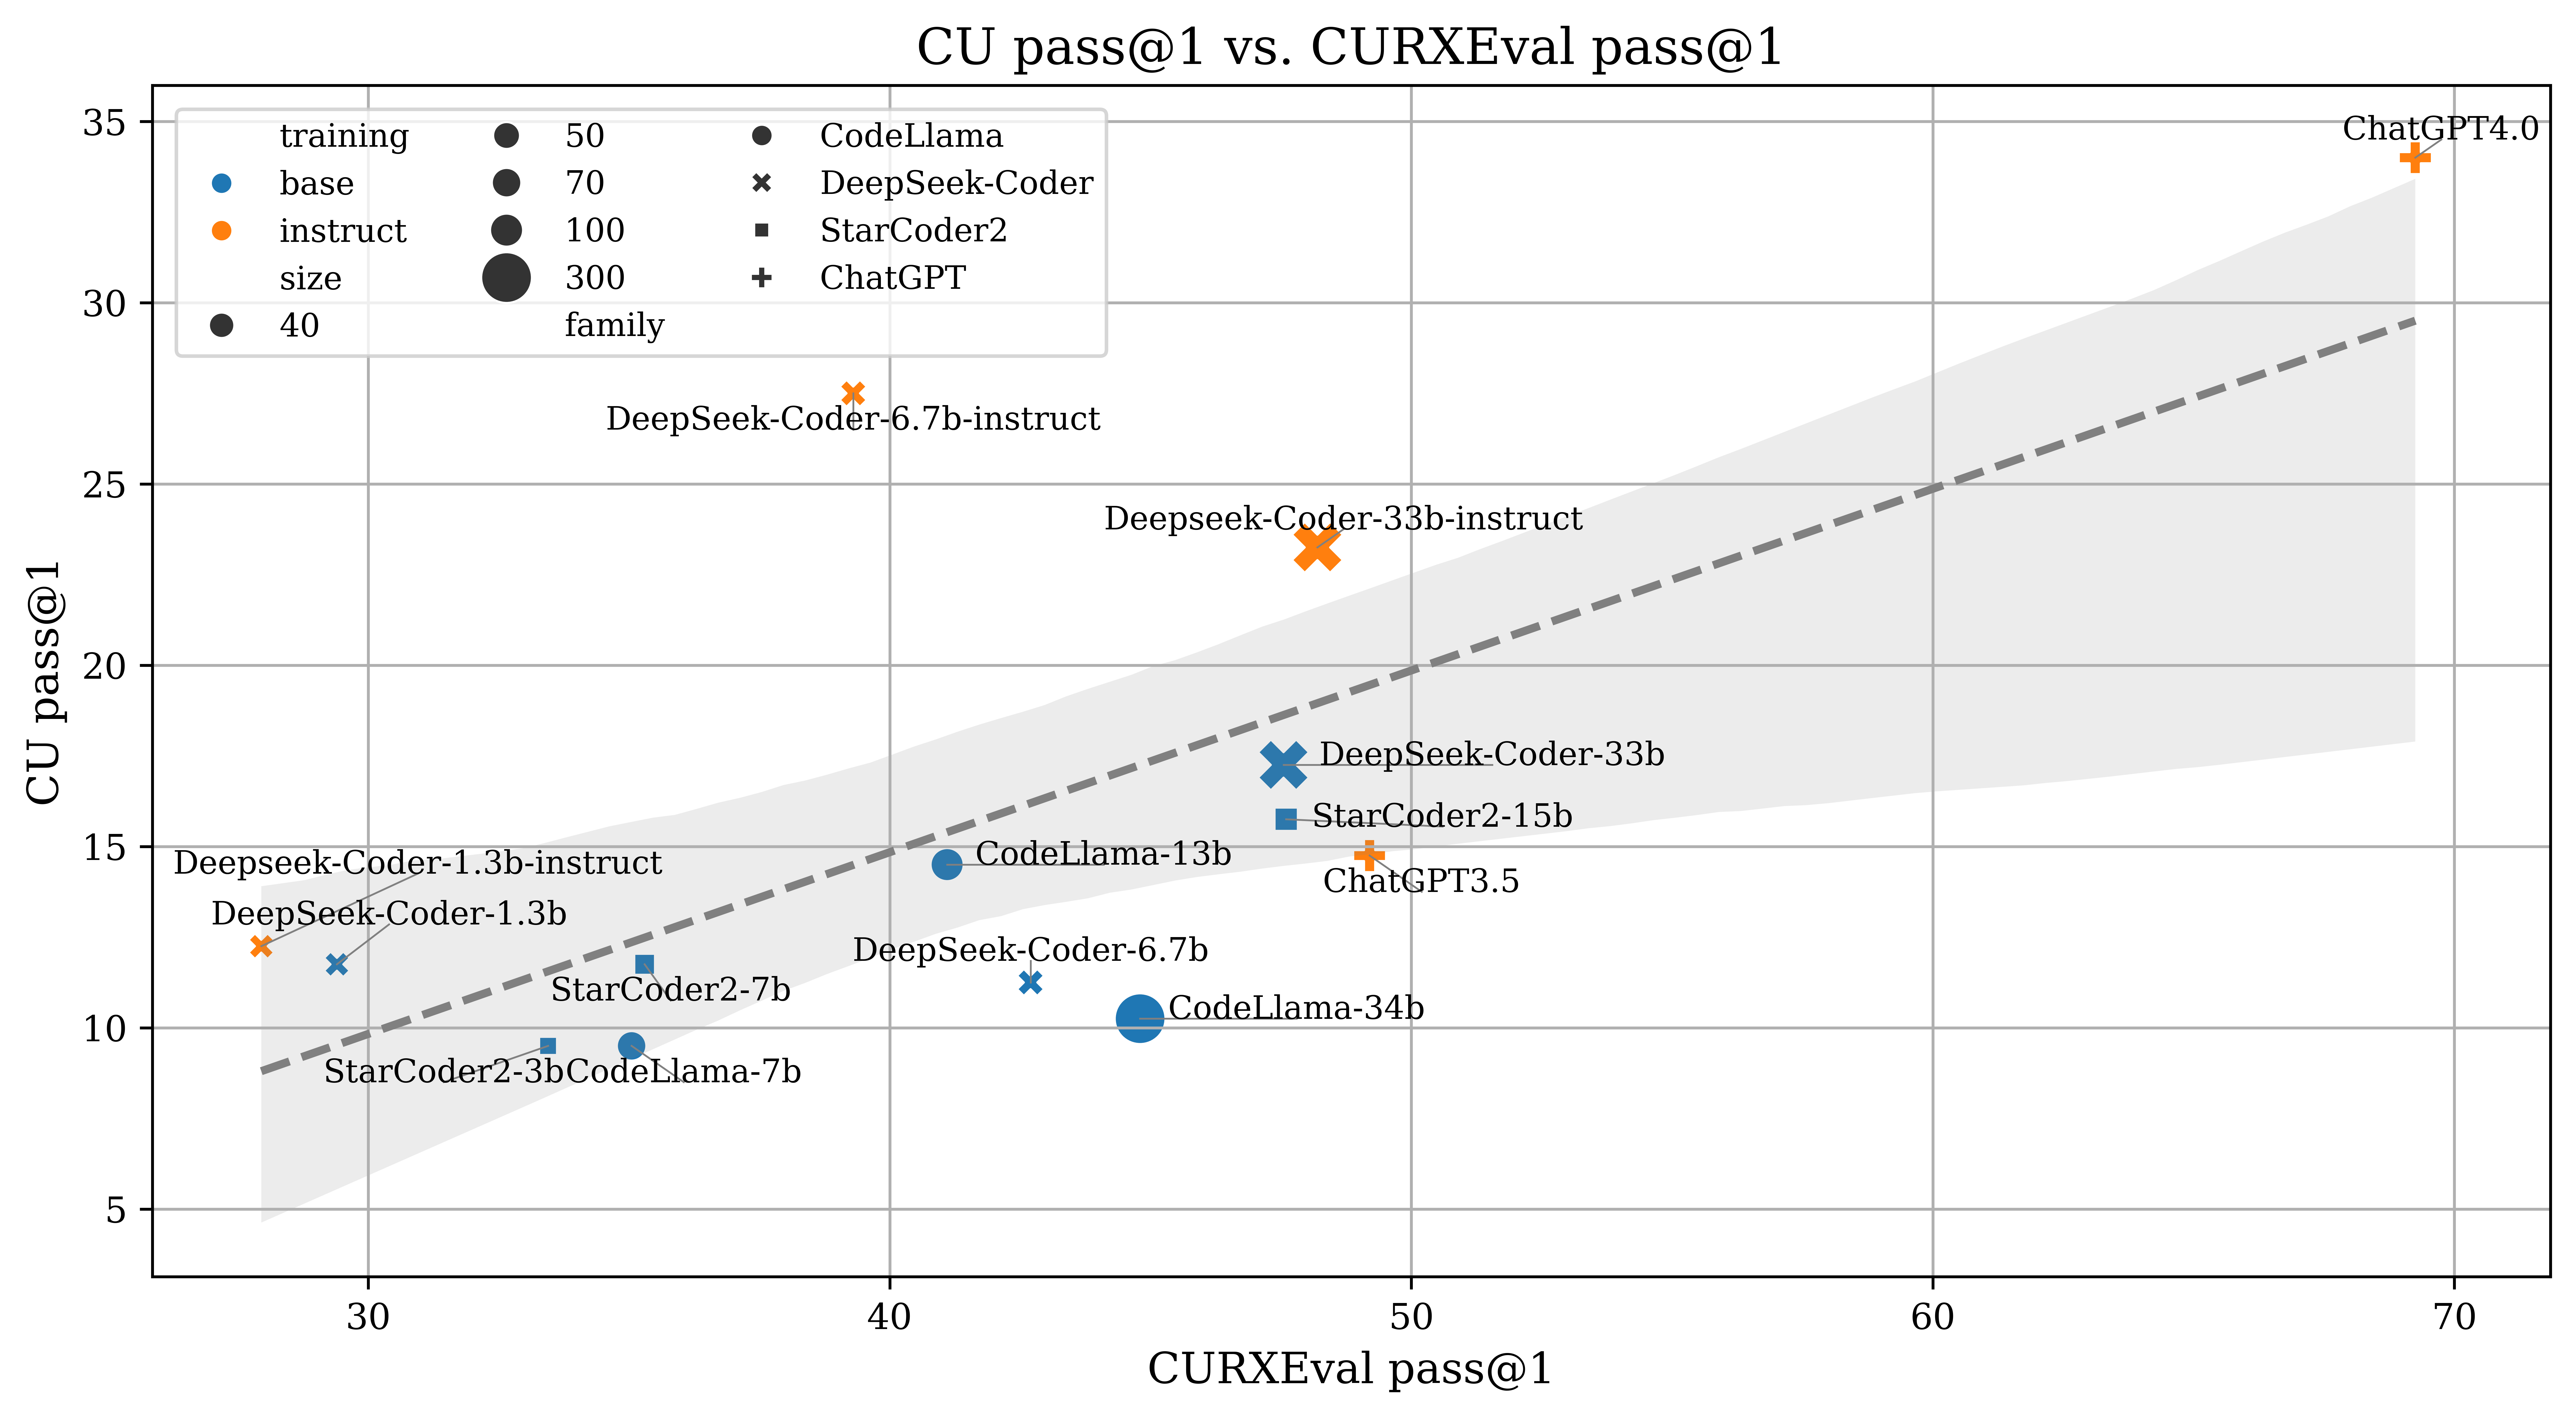}
    \caption{Comparison of CU task pass@1 and CURXEval pass@1 across various models. CURXEval is another benchmark focus on CU task.}
    \label{fig:cor2}
\end{figure}
