# Supplementary material for: CoCo-Bench: A Comprehensive Code Benchmark For Multi-task Large Language Model Evaluation
Source: arXiv:2504.20673 source file (2025-04-29)
Supplement: Supplementary file 2 [file 9_showcase.tex]

\onecolumn
\section{Showcase}
Next, we will show the performance of Code-Llama-13b-hf on some CU samples. As can be observed, all responses were incorrect, indicating a significant challenge for this model in tackling CU task.
\vspace{0.5cm}
\begin{lstlisting}[language=TeX, numbers=none, breaklines=false]
(*@\textbf{Prefix prompt for \texttt{$\mathrm{CU_{R}}$ }:}@*)
description: 
"""Given an array of integers nums and an integer target, return indices of the two numbers 
   such that they add up to target.
You may assume that each input would have exactly one solution, and you may not use
the same element twice.You can return the answer in any order."""
code:
"""
class Solution {
    public int[] twoSum(int[] nums, int target) {
        int n = nums.length;
        for (int i = 0; i < n; ++i) {
            for (int j = i + 1; j < n; ++j) {
                if (nums[i] + nums[j] == target) {
                    return new int[]{i, j};
                }
            }
        return new int[0];
        }
    }
"""
input: nums = [2, 7, 11, 15], target = 9
expected_output: [0, 1]
metadata : 
"""
    programming_language: Java,
    difficulty: Beginner,
    test_aspect: Algorithm
"""
\end{lstlisting}
\begin{lstlisting}[language=TeX, numbers=none, breaklines=false]
(*@\textbf{Response generated by Code-Llama-13b-hf on \texttt{$\mathrm{CU_{F}}$ task }:}@*)
{
    "code": 
        "class Solution {    
            public int[] twoSum(int[] nums, int target) 
            {        
                int n = nums.length;        
                for (int i = 0; i < n; ++i) {            
                for (int j = i + 1; j < n; ++j) 
                {                
                    if (nums[i] + nums[j] == target) 
                    {         
                        return new int[]{i, j};                
                    }            
                }        
            }        
                return new int[0];    
            }
        }", 
    "input": 
        "{'nums': [2, 7, 11, 15], 'target': 9}",
    "output": 
        "[1, 10]"
}
\end{lstlisting}
\begin{lstlisting}[language=TeX, numbers=none, breaklines=false]
(*@\textbf{Response generated by Code-Llama-13b-hf on \texttt{$\mathrm{CU_{R}}$ task }:}@*)
"{
    "code": 
        "class Solution {    
            public int[] twoSum(int[] nums, int target) {        
                int n = nums.length;        
                for (int i = 0; i < n; ++i) {            
                    for (int j = i + 1; j < n; ++j) {                
                        f (nums[i] + nums[j] == target) {                    
                            return new int[]{i, j};                
                        }                    
                    }        
                return new int[0];    
                }
            }", 
    "input": 
        "{'nums': [1, 5, 3, 6, 7], 'target': 1}", 
    "output": "[0, 1]"
}"


\end{lstlisting}

\noindent
\vspace{0.5cm}
The following is a response generated by GPT-4 on a sample of CG task.
\vspace{0.5cm}
\begin{lstlisting}[language=TeX, numbers=none, breaklines=false]
(*@\textbf{An example of \texttt{$\mathrm{CG}$ task}:}@*)
description: """You are given a 0-indexed 2D matrix grid of size m x n, 
where (r, c) represents:A land cell if grid[r][c] = 0, or 
A water cell containing grid[r][c] fish, if grid[r][c] > 0.
A fisher can start at any water cell (r, c) and can do the following operations 
any number of times:Catch all the fish at cell (r, c), or 
Move to any adjacent water cell. Return the maximum number of fish the 
fisher can catch if he chooses his starting cell optimally, 
or 0 if no water cell exists.An adjacent cell of the cell (r, c), 
is one of the cells (r, c + 1), (r, c - 1), (r + 1, c) or (r - 1, c) if it exists.
"""
incomplete_code
"""
class Solution {
    static constexpr int dirs[4][2] = {{-1, 0}, {1, 0}, {0, -1}, {0, 1}};
public:
    int findMaxFish(vector<vector<int>> &grid) {
        int m = grid.size(), n = grid[0].size(), ans = 0;
        function<int(int, int)> dfs = [&](int x, int y) -> int {
            if (____)
                return 0;
        int sum = grid[x][y];
        grid[x][y] = 0; 
        for (auto &d: dirs) 
            ____
        return sum;
    };
        for (int i = 0; i < m; ++i)
            for (int j = 0; j < n; ++j)
                ans = max(ans, dfs(i, j));
        
        return ans;
    }
};
"""
complete_code
class Solution {
    static constexpr int dirs[4][2] = {{-1, 0}, {1, 0}, {0, -1}, {0, 1}};
public:
    int findMaxFish(vector<vector<int>> &grid) {
        int m = grid.size(), n = grid[0].size(), ans = 0;
        function<int(int, int)> dfs = [&](int x, int y) -> int {
            if (x < 0 || x >= m || y < 0 || y >= n || grid[x][y] == 0)
                return 0;
            int sum = grid[x][y];
            grid[x][y] = 0; 
            for (auto &d: dirs) 
                sum += dfs(x + d[0], y + d[1]);
            return sum;
        };
        for (int i = 0; i < m; ++i)
            for (int j = 0; j < n; ++j)
                ans = max(ans, dfs(i, j));
        return ans;
    }
};
input: grid = [[0,2,1,0],[4,0,0,3],[1,0,0,4],[0,3,2,0]]
expected_output: 7
metadata : 
"""
    programming_language: cpp,
    difficulty: Medium,
    test_aspect: Algorithm Integration and Code Completion
"""
\end{lstlisting}
\begin{lstlisting}[language=TeX, numbers=none, breaklines=false]
(*@\textbf{Response generated by GPT-4 on \texttt{$\mathrm{CG}$ task }:}@*)
{
    "complete_code": "
    class Solution {
        static constexpr int dirs[4][2] = {{-1, 0}, {1, 0}, {0, -1}, {0, 1}};

    public:
        int findMaxFish(vector<vector<int>> &grid) {
            int m = grid.size(), n = grid[0].size(), ans = 0;

            function<int(int, int)> dfs = [&](int x, int y) -> int {
                if (x < 0 || x >= m || y < 0 || y >= n || grid[x][y] == 0) 
                    return 0;
                int sum = grid[x][y];
                grid[x][y] = 0;
                for (auto &d: dirs) {
                    int nx = x + d[0], ny = y + d[1];
                    sum += dfs(nx, ny);
                }
                return sum;
            };

            for (int i = 0; i < m; ++i)
                for (int j = 0; j < n; ++j)
                    if (grid[i][j] > 0) 
                        ans = max(ans, dfs(i, j));

            return ans;
        }
    };"
}

\end{lstlisting}

\vspace{0.5cm}
The following is a correct response generated by GPT-4 on a sample of CG task.
\vspace{0.5cm}
\begin{lstlisting}[language=TeX, numbers=none, breaklines=false]
(*@\textbf{An example of \texttt{$\mathrm{CG}$ task}:}@*)
description: """You are given a 0-indexed 2D matrix grid of size m x n, 
where (r, c) represents:A land cell if grid[r][c] = 0, or 
A water cell containing grid[r][c] fish, if grid[r][c] > 0.
A fisher can start at any water cell (r, c) and can do the following operations 
any number of times:Catch all the fish at cell (r, c), or 
Move to any adjacent water cell. Return the maximum number of fish the 
fisher can catch if he chooses his starting cell optimally, 
or 0 if no water cell exists.An adjacent cell of the cell (r, c), 
is one of the cells (r, c + 1), (r, c - 1), (r + 1, c) or (r - 1, c) if it exists.
"""
incomplete_code
"""
class Solution {
    static constexpr int dirs[4][2] = {{-1, 0}, {1, 0}, {0, -1}, {0, 1}};
public:
    int findMaxFish(vector<vector<int>> &grid) {
        int m = grid.size(), n = grid[0].size(), ans = 0;
        function<int(int, int)> dfs = [&](int x, int y) -> int {
            if (____)
                return 0;
        int sum = grid[x][y];
        grid[x][y] = 0; 
        for (auto &d: dirs) 
            ____
        return sum;
    };
        for (int i = 0; i < m; ++i)
            for (int j = 0; j < n; ++j)
                ans = max(ans, dfs(i, j));
        
        return ans;
    }
};
"""
complete_code
class Solution {
    static constexpr int dirs[4][2] = {{-1, 0}, {1, 0}, {0, -1}, {0, 1}};
public:
    int findMaxFish(vector<vector<int>> &grid) {
        int m = grid.size(), n = grid[0].size(), ans = 0;
        function<int(int, int)> dfs = [&](int x, int y) -> int {
            if (x < 0 || x >= m || y < 0 || y >= n || grid[x][y] == 0)
                return 0;
            int sum = grid[x][y];
            grid[x][y] = 0; 
            for (auto &d: dirs) 
                sum += dfs(x + d[0], y + d[1]);
            return sum;
        };
        for (int i = 0; i < m; ++i)
            for (int j = 0; j < n; ++j)
                ans = max(ans, dfs(i, j));
        return ans;
    }
};
input: grid = [[0,2,1,0],[4,0,0,3],[1,0,0,4],[0,3,2,0]]
expected_output: 7
metadata : 
"""
    programming_language: cpp,
    difficulty: Medium,
    test_aspect: Algorithm Integration and Code Completion
"""
\end{lstlisting}
\begin{lstlisting}[language=TeX, numbers=none, breaklines=false]
(*@\textbf{Response generated by GPT-4 on \texttt{$\mathrm{CG}$ task }:}@*)
{
    "complete_code": "
    class Solution {
        static constexpr int dirs[4][2] = {{-1, 0}, {1, 0}, {0, -1}, {0, 1}};

    public:
        int findMaxFish(vector<vector<int>> &grid) {
            int m = grid.size(), n = grid[0].size(), ans = 0;

            function<int(int, int)> dfs = [&](int x, int y) -> int {
                if (x < 0 || x >= m || y < 0 || y >= n || grid[x][y] == 0) 
                    return 0;
                int sum = grid[x][y];
                grid[x][y] = 0;
                for (auto &d: dirs) {
                    int nx = x + d[0], ny = y + d[1];
                    sum += dfs(nx, ny);
                }
                return sum;
            };

            for (int i = 0; i < m; ++i)
                for (int j = 0; j < n; ++j)
                    if (grid[i][j] > 0) 
                        ans = max(ans, dfs(i, j));

            return ans;
        }
    };"
}

\end{lstlisting}

\vspace{0.5cm}
The following is a correct response that passes all the test cases, showcasing the capability of DeepSeek-Coder-6.7b. This output was generated on a challenging sample of the CM task, demonstrating the model's proficiency in handling complex coding problems.
\vspace{0.5cm}

\begin{lstlisting}[language=TeX, numbers=none, breaklines=false]
(*@\textbf{An example of \texttt{$\mathrm{CM}$ task }:}@*)
"""You are given an array nums of non-negative integers and an integer k.
An array is called special if the bitwise or of all of its elements is at least k.
Return the length of the shortest special non-empty subarray of nums, 
or return -1 if no special subarray exists."""
buggy_code
"""
class Solution:    
    def minimumSubarrayLength(self, nums: List[int], for: int) -> int:
        res = 51
        n = len(nums)
        for i in range(n):
            for j in range(i, n):
                sum_or = 0
                for idx in range(i, j + 1): sum_or |= nums[idx]
                if sum_or >= k: res = min(res, j - i + 1)
        return res if res != 51 else -1
"""
input: nums = [2, 1, 8], k = 10
expected_output: 3
execution_returns: 
line 2 def minimumSubarrayLength(self, nums: List[int], for: int) -> int:   
SyntaxError: invalid syntax
metadata : 
"""
    programming_language: Python,
    difficulty: Intermediate,
    test_aspect: Algorithm Debugging
"""
\end{lstlisting}
\begin{lstlisting}[language=TeX, numbers=none, breaklines=false]
(*@\textbf{The response from DeepSeek-Coder-6.7b on \texttt{$\mathrm{CM}$ task }:}@*)
class Solution:
    def minimumSubarrayLength(self, nums: List[int], k: int) -> int:
        res = float('inf')
        n = len(nums)
        sum_or = 0
        left = 0
        for right in range(n):
            sum_or |= nums[right]
            while sum_or >= k:
                res = min(res, right - left + 1)
                sum_or ^= nums[left]
                left += 1
        return res if res != float('inf') else -1
\end{lstlisting}
% \vspace{0.5cm}
% The following is a correct response that passes all the test cases, showcasing the capability of DeepSeek-Coder-6.7b. This output was generated on a challenging sample of the CM task, demonstrating the model's proficiency in handling complex coding problems.
% \vspace{0.5cm}
% \begin{lstlisting}[language=TeX, numbers=none, breaklines=false]
% (*@\textbf{An example of \texttt{$\mathrm{CM}$ task }:}@*)
% """You are given an array nums of non-negative integers and an integer k.
% An array is called special if the bitwise or of all of its elements is at least k.
% Return the length of the shortest special non-empty subarray of nums, 
% or return -1 if no special subarray exists."""
% buggy_code
% """
% class Solution:    
%     def minimumSubarrayLength(self, nums: List[int], for: int) -> int:
%         res = 51
%         n = len(nums)
%         for i in range(n):
%             for j in range(i, n):
%                 sum_or = 0
%                 for idx in range(i, j + 1): sum_or |= nums[idx]
%                 if sum_or >= k: res = min(res, j - i + 1)
%         return res if res != 51 else -1
% """
% input: nums = [2, 1, 8], k = 10
% expected_output: 3
% execution_returns: 
% line 2 def minimumSubarrayLength(self, nums: List[int], for: int) -> int:   
% SyntaxError: invalid syntax
% metadata : 
% """
%     programming_language: Python,
%     difficulty: Intermediate,
%     test_aspect: Algorithm Debugging
% """
% \end{lstlisting}
% \begin{lstlisting}[language=TeX, numbers=none, breaklines=false]
% (*@\textbf{The response from DeepSeek-Coder-6.7b on \texttt{$\mathrm{CM}$ task }:}@*)
% class Solution:
%     def minimumSubarrayLength(self, nums: List[int], k: int) -> int:
%         res = float('inf')
%         n = len(nums)
%         sum_or = 0
%         left = 0
%         for right in range(n):
%             sum_or |= nums[right]
%             while sum_or >= k:
%                 res = min(res, right - left + 1)
%                 sum_or ^= nums[left]
%                 left += 1
%         return res if res != float('inf') else -1
% \end{lstlisting}
\vspace{0.5cm}
The following is an example of a CR generated by DeepSeek-Coder-6.7b-Instruct, with all classifications correctly identified.
\vspace{0.5cm}

\begin{lstlisting}[language=TeX, numbers=none, breaklines=false]
(*@\textbf{An example of \texttt{$\mathrm{CR}$ task }:}@*)
"""Function is designed to fetch data from a URL provided by the user, process it, 
and return a modified result. 
It contains multiple categories of errors, including syntax, 
logic, performance, and security issues."""
# code
"""
def fetch_and_process_data(user_url):
    import requests
    data = request.get(user_url)
    processed_data = []
    if data.status_code == 200:
        content = data.json()
        for item in content['results']:
            if type(item) is str:
                processed_data.append(item.lower()) 
            else:
                continue  
    else:
        print('Failed to fetch data')
    eval('print(processed_data)') 
    return processed_data
"""
issue_categories
"""
    syntax_errors: data = request.get(user_url)
    logical_errors: continue
    performance_issues: processed_data.append(item.lower())
    security_issues: eval('print(processed_data)')
"""
metadata : 
"""
    programming_language: Python,
    difficulty: Advanced,
    test_aspect: Comprehensive Error Analysis
"""
\end{lstlisting}
\begin{lstlisting}[language=TeX, numbers=none, breaklines=false]
(*@\textbf{The response from DeepSeek-Coder-6.7b-Instruct}@*)
{
    "performance_issues": 
            "processed_data.append(item.lower()) ",
    "security_issues": 
            "eval('print(processed_data)') ,
    "irregular_naming": "None",
    "logical_errors": "continue"
}
\end{lstlisting}
\twocolumn
